# Supplementary material for: Robust and differentially private stochastic linear bandits
Source: arXiv:2304.11741 source file (2023-04-23)
Supplement: Supplementary file 1 [file robust_estimation.tex]

\section{A robust algorithm for batched bandits}

The phased arm elimination algorithm with local differential privacy and
robustness to adversarial contamination is given below.

\begin{algorithm}[h]
    \caption{Robust DP arm elimination}
    \begin{algorithmic}[1]
        \State \textbf{Input}: action space $\cA$, $T$, $B$,
        failure prob. $\delta$, variance $\sigma^2$,
        corruption prob. $\alpha \in (0, 1/4)$.
        \State Set $\cA_0 := \cA$, $q = T^{1/B}$
        \For{$i = 1, \dots, B - 1$}
            \State Set $\varepsilon_i := \sqrt{\frac{d \log (1 / \delcore)}{q^i}}$.
            \State Form a coreset $\cS_{\cA_{i-1}}$ with
            $n_i = \Theta(d \log(1 / \delcore) / \varepsilon_i^2)$ elements.
            \State Play actions $a_j \in \cS_{\cA_{i-1}}$ and observe rewards $r_j$
            according to~\eqref{eq:noise-model}.
            \State Compute $\widehat{w}_i :=
            \mathtt{RobustLeastSquares}(\set{a_j}, \set{r_j}, \alpha)$.
            \label{op:robust-lsq-est}
            \State Set the elimination threshold
            \[
                \gamma_i := C \left( \alpha \sigma \sqrt{d} + \sqrt{\sigma d}
                    \max\set{
                        \alpha, \frac{\log(\frac{n_i + d}{\delta})}{n_i}
                    }^{1/2} +
                    \sigma \sqrt{\frac{d^2 + d \log(1 / \delta)}{n_i}}
                \right)
            \]
            \State Eliminate suboptimal arms:
            \[
                \cA_{i} := \set{
                    a \in \cS_{\cA_{i-1}} \mid
                    \langle a, \widehat{w}_i\rangle \geq
                    \max_{a' \in \cS_{\cA_{i-1}}} \langle a', \widehat{w}_i \rangle
                    - 2 \gamma_i
                }.
            \]
        \EndFor
        \State Play the ``best'' action in $\cS_{\cA_{B-1}}$ in the last round.
    \end{algorithmic}
    \label{alg:arm-elimination-robust}
\end{algorithm}
\subsection{Robust estimation of the least-squares solution}
In this section, we describe how to estimate the least-squares solution robustly.
In particular, we are interested in solving the problem
\begin{equation}
    \min_{\theta} \frac{1}{n} \sum_{i = 1}^n \left(\ip{\theta, a_i} - \ip{\theta^{\star}, a_i}\right)^2,
\end{equation}
when our observations follow the model laid forth in the introduction.
\begin{assumption} \label{assumption:least-squares-estimation}
The following assumptions hold:
\begin{enumerate}
    \item The probability of corruption $\alpha$ in the current round satisfies
    \[
        \alpha < \frac{1}{4}.
    \]
    \item The number of samples in the current round satisfies
    \[
        n \gtrsim \frac{\log(\min(n, d) / \delta)}{\alpha}.
    \]
    \item The matrix of covariates $M := \sum_{ i = 1 }^n a_i a_i^{\T}$ is invertible.
    \item The covariates and unknown parameter satisfy $\norm{a_i} \leq 1$ and $\norm{\theta^{\star}} \leq 1$.
\end{enumerate}
\end{assumption}
We also let $\set{a_1, \dots, a_n}$ be a G-optimal design with error level $\varepsilon$,
so that the least squares estimate
\begin{equation}
    \widehat{\theta} := M^{-1} \sum_{i = 1}^n a_i y_i
    \label{eq:least-squares-error}
\end{equation}
satisfies $\bigip{a, \widehat{\theta} - \theta^{\star}} \leq \varepsilon$ with high probability
for all $a \in \cA$.

We will use the \textsc{Scram} algorithm from~\cite{CMY22}. The setting is as follows: consider
\begin{equation}
    y_i = y_i^{\star} + \xi_i, \quad y_i^{\star} = \ip{a_i, \theta^{\star}} + \epsilon_i, \; \;
    \xi_i \sim \cD
    \label{eq:scram-measurement-setup}
\end{equation}
for some subgaussian distribution $\cD$ with variance $\sigma^2$ and misspecification errors
$\epsilon_i$ satisfying
\begin{equation}
  \frac{1}{n} \sum_{i = 1}^n \epsilon_i^2 \leq \epsilon^2, \quad
  \text{for some $\epsilon \in \Rbb_+$}.
  \label{eq:avg-misspecification}
\end{equation}
Given a radius $R > 0$, we define the ``oracle'' estimator
\begin{equation}
    u^{\star} = \arg\min_{\norm{u} \leq R} \frac{1}{n}
    \sum_{i = 1}^n \left(\ip{u, a_i} - y_i^{\star} \right)^2,
    \label{eq:constrained-ls}
\end{equation}
Moreover, let $M_n$ denote the empirical second moment matrix:
\begin{equation}
    M_n := \frac{1}{n} \sum_{i = 1}^n a_i a_i^{\T}.
    \label{eq:empirical-second-moment-matrix}
\end{equation}
We want to make use of the \textsc{Scram} estimator from~\cite{CMY22} to estimate
$u^{\star}$ from~\eqref{eq:constrained-ls} robustly. The guarantees of that estimator
are summarized below:
\begin{theorem}[{\cite[Theorem 5.13]{CMY22}}]
    \label{theorem:scram}
    Suppose~\cref{assumption:least-squares-estimation} holds.
    There is a polynomial-time algorithm that computes an estimate $\widehat{w}$
    satisfying
    \begin{equation}
        \norm{\widehat{w} - u^{\star}}_{M_n} \leq \begin{aligned}[t]
        & \alpha \sigma + \epsilon \sqrt{\alpha} + \left( \alpha^{3/8} \sqrt{R \sigma} + \alpha^{1/8} \sqrt{R \epsilon} \right) \left(
            \frac{\log(\frac{n + d}{\delta})}{n}
        \right)^{1/8} \\
        & + R \alpha^{1/4} \left(
            \frac{\log(\frac{n + d}{\delta})}{n}
        \right)^{\frac{1}{4}} +
        \min\set{
            \sigma \sqrt{\frac{d + \log(1 / \delta)}{n}},
            (R\sigma)^{1/2} \left(\frac{\log(1 / \delta)}{n}\right)^{1/4}
        }
        \end{aligned}
    \end{equation}
    with probability at least $1 - \delta$, where $u^{\star}$ is the estimate
    from~\eqref{eq:constrained-ls} and $M_{n}$ is defined in~\eqref{eq:empirical-second-moment-matrix}.
\end{theorem}

To invoke~\cref{theorem:scram}, we will set $R$ appropriately.
\begin{lemma}
    \label[lemma]{lemma:constrained-ls-solution}
    Suppose that $\epsilon = 0$ in~\eqref{eq:avg-misspecification} and $M_n$ is
    invertible. Then for $R > 1$, we have $u^{\star} = \theta^{\star}$.
\end{lemma}
\begin{proof}
    The first-order optimality conditions for the convex program in~\eqref{eq:constrained-ls}
    read
    \begin{align*}
        0 &\in \frac{2}{n} \sum_{i = 1}^n a_i (\ip{u^{\star}, a_i} - y_i^{\star})
          + N_{\cB(0; R)}(u^{\star}) \\
          &= \frac{2}{n} \sum_{i = 1}^n a_i a_i^{\T} (u^{\star} - \theta^{\star})
          + N_{\cB(0; R)}(u^{\star}),
    \end{align*}
    where $N_{\cB(0; R)}(x)$ is the normal cone to $\cB(0; R)$ at $x$.
    Since $M_n$ is invertible by~\cref{assumption:least-squares-estimation}, the
    objective in~\eqref{eq:constrained-ls} is strictly convex and admits a unique
    solution. Finally, since $\norm{\theta^{\star}} \leq 1$ and $R > 1$, we have
    $N_{\cB(0; R)}(\theta^{\star}) = 0$ and thus $u^{\star} = \theta^{\star}$
    satisfies the first-order optimality condition.
\end{proof}
We now consider the construction of confidence intervals. In particular, we have
\begin{align*}
    \abs{\ip{a, \widehat{w} - \theta^{\star}}}
    &\leq
    \norm{a}_{M_n^{-1}} \norm{\widehat{w} - u^{\star}}_{M_n}
    =
    \norm{a}_{M_n^{-1}} \norm{\widehat{w} - \theta^{\star}}_{M_n},
\end{align*}
using the Cauchy-Schwarz inequality. We upper bound the first term using
$$
\norm{a}_{M_n^{-1}} = \sqrt{\ip{a, \left(\frac{1}{n} \sum_{i = 1}^n a_i a_i^{\T}\right)^{-1} a}} = \sqrt{n} \| a \|_{M^{-1}} \leq
\varepsilon \sqrt{\frac{n}{\log(1 / \delta)}} = \sqrt{d},
$$
where the first inequality follows from~\cref{lemma:g-optimal-design-norm-bound} and the
last equality follows from the fact that a $G$-optimal design has
$n = \frac{d \log(1 / \delta)}{\varepsilon^2}$. For the second term, we
invoke~\cref{theorem:scram,lemma:constrained-ls-solution} to arrive at
\[
    \norm{\widehat{w} - \theta^{\star}} \lesssim
    \begin{aligned}[t]
    & \alpha \sigma + \sqrt{\sigma} \alpha^{3/8} \left(
        \frac{\log(\frac{n + d}{\delta})}{n}^{1/8}
    \right) +
    \alpha^{1/4} \left(
        \frac{\log(\frac{n + d}{\delta})}{n}
    \right)^{1/4} \\
    & +
    \min\set{
        \sigma \sqrt{\frac{d + \log(1 / \delta)}{n}},
        \sqrt{\sigma} \left(\frac{\log(1 / \delta)}{n}\right)^{1/4}
    }.
    \end{aligned}
\]
Finally, we arrive at a compact description by assuming $\sigma \ge 1$ and
merging common terms.
\begin{corollary}
    \label[corollary]{corollary:confidence-interval}
    Suppose~\cref{assumption:least-squares-estimation} holds, $\sigma \geq 1$, and
    $\epsilon = 0$.
    Then there is a polynomial time algorithm computing an estimate $\widehat{w}$
    such that, with probability at least $1 - 2\delta$, we have
    \begin{equation}
        \max_{a \in \cA}\abs{\ip{a, \widehat{w} - \theta^{\star}}}
        \lesssim
        \alpha \sigma \sqrt{d} + \sqrt{\sigma d} \max\set{
            \alpha, \left(\frac{\log(\frac{n + d}{\delta})}{n}\right)
        }^{1/2} +
        \sigma \sqrt{\frac{d^2 + d\log(1 / \delta)}{n}}
    \end{equation}
\end{corollary}

\subsection{Regret analysis}
\label{sec:regret-analysis}
We condition on the ``good'' event where all calls to the coreset construction
and \textsc{Scram} succeed. Since that event fails with probability at most $O(T \delta)$,
we will eventually relabel $\delta := \frac{\delta}{T^2}$. On that event, we can
prove the following:

\paragraph{The optimal arm is not eliminated.}
Let $a^{\star}$ be the arm maximizing $\ip{a, \theta^{\star}}$ over all $a \in \cA$. Then for any $a \in \cA$, we have
\begin{align*}
    \bigip{a, \widehat{w}} - \bigip{a^{\star}, \tilde{\theta}} &=
    \ip{a, \theta^{\star}} - \ip{a^{\star}, \theta^{\star}} -
    \left(\bigip{a, \widehat{w} - \theta^{\star}} -
          \bigip{a^{\star}, \widehat{w} - \theta^{\star}}\right) \\
    &\leq \ip{a - a^{\star}, \theta^{\star}} + 2 \gamma_i
    \leq 2 \gamma_i,
\end{align*}
using~\cref{corollary:confidence-interval} in the first inequality and optimality of $a^{\star}$ in the second inequality.

\paragraph{Surviving arms have bounded gap.} Fix any arm $a \in \cA$
and denote its reward gap by $\Delta_{a} := \ip{a^{\star} - a, \theta^{\star}}$.
Then, it follows that
\begin{align}
    \ip{a^{\star} - a, \widehat{w}} &=
    \ip{a^{\star}, \theta^{\star}} + \ip{a^{\star}, \widehat{w} - \theta^{\star}}
  + \ip{a, \theta^{\star} - \widehat{w}} - \ip{a, \theta^{\star}} \notag \\
  &\geq
    \ip{a^{\star} - a, \theta^{\star}} - 2 \gamma_i \notag \\
  &\geq \Delta_{a} - 2 \gamma_i.
  \label{eq:bounded-gap-1}
\end{align}
Now, let $i$ be the smallest index for which $\gamma_i <
\frac{\Delta_{a}}{4}$. Combined with~\eqref{eq:bounded-gap-1}, that implies
\begin{equation*}
    \ip{a^{\star} - a, \theta^{\star}} \geq 2 \gamma_i.
\end{equation*}
Consequently, any arm with gap $\Delta_{a} > 4 \gamma_i$ for some index $i$ will be
eliminated at round $i$. Equivalently, all active arms at the beginning of
round $i$ must satisfy
\begin{equation}
    \Delta_{a} \leq 4 \gamma_{i - 1}, \; \;
    \text{for all $a \in \cA_{i-1}$.}
    \label{eq:bounded-gap-2}
\end{equation}
Putting all ingredients together, the expected regret conditioned on the
``good'' event is given by
\begin{align}
R_T &= \sum_{i = 1}^B
(\text{arms pulled}) \times (\text{instantaneous regret}) \notag \\
&=
\sum_{i = 1}^B n_i \cdot 4 \gamma_{i-1} \notag \\
&\lesssim 4 \sum_{i = 1}^B q^i \left(
\alpha \sigma \sqrt{d} + \sqrt{\sigma d} \max\left\{
\sqrt{\alpha}, \left(
\frac{\log(\frac{q^{i - 1} + d}{\delta})}{q^{i-1}}
\right)^{1/2}
\right\}
+ \sigma \sqrt{\frac{d^2 + d \log(1 / \delta)}{q^{i-1}}}
\right) \notag \\
&\leq
4 \sum_{i = 1}^B q^i \left(
  \alpha \sigma \sqrt{d} + \sqrt{\sigma d}
  \max\left(\alpha, \frac{\log(\frac{T + d}{\delta})}{q^{i-1}}\right)^{1/2}
  + \sigma \sqrt{\frac{d^2 + d \log(1 / \delta)}{q^{i-1}}}
\right).
\label{eq:regret-master}
\end{align}
We analyze each term separately. The first term yields
\begin{equation}
4 \sum_{i = 1}^B q^i \alpha \sigma \sqrt{d} = 4 \alpha \sigma \sqrt{d} \cdot T.
\label{eq:regret-first}
\end{equation}
The first part of the second term yields
\begin{equation}
4 \sqrt{\sigma d \alpha} \sum_{i = 1}^B q_i =
4 \sqrt{\sigma d \alpha} \cdot T.
\label{eq:regret-second-i}
\end{equation}
The second part of the second term yields
\begin{align}
& q \sqrt{\sigma d \log\left(\frac{T + d}{\delta}\right)} \sum_{i = 1}^B \sqrt{q^{i - 1}} \notag \\
&=
q \sqrt{\sigma d} \left( \sqrt{\log(qd)} \sum_{j = 0}^{B-1} \sqrt{j} q^{j / 2}
+
\sqrt{\log(1 / \delta)} \sum_{j = 0}^{B-1} q^{j/2}
\right) \notag \\
&\leq
q \sqrt{\sigma d \log(qd)} \sqrt{B} \cdot \frac{\sqrt{q}^{B} - 1}{\sqrt{q} - 1}
+ q \sqrt{\sigma d \log(1 / \delta)} \cdot \frac{\sqrt{q}^{B} - 1}{\sqrt{q} - 1}.
\label{eq:regret-second-ii}
\end{align}
Finally, the last term satisfies
\begin{align}
\sum_{i = 1}^B q^i \sigma \sqrt{\frac{d^2 + d \log(1 / \delta)}{q^{i-1}}} &=
q \sigma \sqrt{(d^2 + d \log(1 / \delta))} \sum_{j = 0}^{B - 1} \sqrt{q}^{j} \\
&=
q \sigma \sqrt{\left(d^2 + d \log(1 / \delta)\right)} \cdot
\frac{\sqrt{q}^B - 1}{\sqrt{q} - 1}.
\label{eq:regret-third}
\end{align}
Letting $q = T^{1/B}$ and $B \gtrsim \log(T)$, we have
\[
\frac{\sqrt{q}^B - 1}{\sqrt{q} - 1} \asymp \sqrt{T}.
\]
Therefore, collecting~\cref{eq:regret-first,eq:regret-second-i,eq:regret-second-ii,eq:regret-third} we obtain
\begin{align}
    R_T &\lesssim
    \sqrt{d} T \left( \alpha \sigma + \sqrt{\alpha \sigma} \right) +
    \sqrt{\sigma} T^{\frac{1}{2} + B} \left(
        \sqrt{d B \log(T^{1/B} d)} +
        \sqrt{\sigma (d^2 + d \log(1 / \delta))}
    \right).
    \label{eq:regret-bound-good}
\end{align}

\subsection{Robust linear bandits with local differential privacy}
Consider a model where every client wants to privatize their responses.
To do so, client $i$ returns
\begin{equation}
    \bar{r}_i := \cM( r_i ) = \cM(\ip{a_i, \theta^{\star}} + \eta_i),
\end{equation}
where $\eta_i \sim \mathrm{SubG}(1)$ and $\cM(\cdot)$ is a privacy-inducing mechanism.

\begin{lemma}[Local DP via the Gaussian mechanism]
    Let $\cM(x) := x + \xi$ where
    $\xi$ is distributed according to $\cN\left(0, \frac{4\log(1 / \delpriv)}{\epspriv^2}\right)$. Then $\cM(r_i)$ is $(\epspriv,\delpriv)$-locally differentially private
    for all $i$.
\end{lemma}
\begin{proof}
    Since we have $\abs{\ip{a_i, \theta^{\star}}} \leq 1$, the $\ell_2$-sensitivity of
    the reward sequence (and thus the sensitivity of every client) is upper bounded by $2$.
    The claim follows using standard properties of the Gaussian mechanism.
\end{proof}
Notice that the above mechanism implies that all rewards follow the form
\[
    \bar{r}_i = \ip{a_i, \theta^{\star}} + \zeta_i, \quad
    \zeta_i \sim \mathrm{SubG}\left(
        1 + \frac{2 \sqrt{\log(1 / \delpriv)}}{\epspriv}
    \right).
\]
Consequently, we may appeal to~\cref{corollary:confidence-interval} and~\eqref{eq:regret-bound-good} with
\[
    \sigma = 1 + \frac{2 \sqrt{\log(1 / \delpriv)}}{\epspriv}
\]
to obtain a final regret bound that scales as
\begin{equation}
    R_T = \tilde{O}\left(\sqrt{d} T \left(
    \frac{\alpha}{\epspriv} + \sqrt{\frac{\alpha}{\epspriv}}
    \right)\right) +
    \tilde{O}\left(
        \frac{d \sqrt{T}}{\epspriv}
    \right),
    \label{eq:regret-non-aggregate}
\end{equation}
assuming that the privacy term is dominating the constant in $\sigma$.
When $\alpha = 0$ our algorithm recovers the regret bound of~\cite{HGFD22}
for local differential privacy up to logarithmic factors.

\subsection{Local differential privacy with aggregated responses}
We also consider an alternative model where every client ``owns'' a vector $a
\in \cA$. The learner queries client $a$ with a number of desired rewards $n_a$
and client $a$ returns
\begin{equation}
    \hat{r}_{a} = \cM_{a}\left(
    \frac{1}{n_{a}} \sum_{i = 1}^{n_a}
    \ip{a, \theta^{\star}} + \eta_i
    \right) \overset{(d)}{=}
    \cM_{a}\left(
        \ip{a, \theta^{\star}} + \eta^{(a)}
    \right), \quad
    \eta^{(a)} \sim \mathrm{SubG}(\sigma_{a}),
    \label{eq:client-response-aggregate}
\end{equation}
where $\cM_{a}: \Rbb \to \Rbb$ is the privacy mechanism of client $a$ and
$\sigma_{a} \lesssim n_{a}^{-1/2}$ for all $a \in \cA$.

The following Lemma shows that it is sufficient to inject Laplacian noise
to the responses to achieve differential privacy.
\begin{lemma}
    \label{lemma:client-response-aggregate-private}
    Let $\cM_{a}(z) := z + \mathsf{Lap}\left(\frac{2}{n_a \epspriv}\right)$.
    Then the response of client $a$ is $\epspriv$-DP.
\end{lemma}
\begin{proof}
    Define the function $f(r) := \frac{1}{n_a} \sum_{i = 1}^{n_a} r_a^{(i)}$,
    where $r_a^{(i)} = \ip{a, \theta^{\star}} + \eta_i$. Considering a neighboring
    reward sequence $r'$ that only differs in 1 element at index $j$, it is immediate
    that the $\ell_1$-sensitivity of $f$ is $\frac{2}{n_a}$. Therefore, the claim
    follows by properties of the Laplace mechanism.
\end{proof}
We now analyze the phased arm elimination algorithm under the above
response model. Suppose we are given an approximate G-optimal design $\pi$ with
induced coreset $\cS \equiv \cS(\pi)$ satisfying
\[
  \abs{\mathrm{supp}(\cS)} \lesssim d \log(\log d),
  \quad
  g(\pi) \leq 2d.
\]
Given such an optimal design $\pi$, we play each action in the coreset a total of
\[
  n_{a} = \max\set{\pi(a), \nu} \cdot n,
\]
where $n$ is the budget in the current round.
Moreover, denote the privatized rewards absent any subgaussian noise by $\bar{r}_a$:
\[
    \bar{r}_a := \ip{a, \theta^{\star}} + \xi_a, \quad
    \xi_a \sim \mathsf{Lap}\left(
        \frac{2}{n_a \epspriv}
    \right).
\]
We now consider the following ``oracle'' least-squares problem:
\begin{equation}
    u^{\star} =
        \argmin_{u: \norm{u} \leq R} \sum_{a \in \cS} (\ip{a, u} - \bar{r}_a)^2
    \equiv
        \argmin_{u: \norm{u} \leq R} \sum_{a \in \cS} (\ip{a, u - \theta^{\star}} -
    \xi_a)^2
    \label{eq:oracle-least-squares-private}
\end{equation}
Note that~\eqref{eq:oracle-least-squares-private} is an instance of the problem
in~\eqref{eq:scram-measurement-setup}, where
\[
    y_{a} = y_{a}^{\star} + \eta_{a}, \; \;
    y_{a}^{\star} = \ip{a, \theta^{\star}} + \xi_{a}, \quad \text{where} \quad
    \eta_a \sim \mathrm{SubG}(\sigma_{a}).
\]
Recall the definition of the empirical second moment matrix $M_n$
in~\eqref{eq:empirical-second-moment-matrix}. Here, we have
\begin{equation}
  M_{n} = \frac{1}{\abs{\cS}} \sum_{a \in \cS} aa^{\T}.
  \label{eq:empirical-second-moment-matrix-coreset}
\end{equation}
In the forthcoming analysis, we shall condition on the following event:
\begin{equation}
    \cQ := \set{\max_{a \in \cS} \abs{\xi_a} \leq \frac{C \log(\abs{\cS} / \delta)}{\epspriv \min_{a \in \cS} n_{a}}}.
    \label{eq:max-laplacian-event}
\end{equation}
\begin{lemma}
    \label{lemma:max-laplacian-event}
    For the event $\cQ$ defined in~\eqref{eq:max-laplacian-event}, we have that
    \begin{equation}
        \prob{\cQ} \geq 1 - \delta.
    \end{equation}
\end{lemma}
\begin{proof}
    Recall that a Laplacian variable $X \sim \mathsf{Lap}(b)$ is a subexponential random
    variable with parameter $\sigma \asymp b$. In particular, the family $\set{\xi_a}_{a \in \cS}$ satisfies
    \begin{equation}
        \bar{\sigma} := \max_{a \in \cS} \norm{\xi_{a}}_{\psi_1} \leq
        \max_{a \in \cS} \frac{1}{n_{a} \epspriv} =
        \frac{1}{\epspriv \min_{a \in \cS} n_{a}}.
        \label{eq:max-subexp-parameter}
    \end{equation}
    Consequently, a union bound along with~\cite[Proposition 2.7.1]{Vershynin18} yield
    \begin{align}
        \prob{\max_{a \in \cS} \abs{\xi_a} \geq t} &\leq
        \sum_{a \in \cS} \prob{\abs{\xi_a} \geq t}
        \leq
        \abs{\cS} \expfun{
            -\min\set{\frac{t^2}{2 \bar{\sigma}^2}, \frac{t}{2\bar{\sigma}}}
        },
    \end{align}
    where $\bar{\sigma}$ has been defined in~\eqref{eq:max-subexp-parameter}.
    The exponential in the expression above is at most $\delta$ when
    \[
        \min\set{\frac{t^2}{2\bar{\sigma}^2}, \frac{t}{\bar{\sigma}}} \geq \log(1 / \delta)
        \implies t \gtrsim \frac{\log(1 / \delta)}{\epspriv \min_{a \in \cS} n_{a}}
    \]
    Setting $\delta := \frac{\delta}{\abs{\cS}}$ completes the proof and relabelling
    completes the proof.
\end{proof}

The next Lemma controls the squared misspecification error for $u^{\star}$.
\begin{lemma}[Misspecification error]
  \label{lemma:misspecification-error}
  For $R = 2$, the average misspecification error of $u^{\star}$ satisfies
  \[
      \epsilon =
      \sqrt{
        \frac{1}{\abs{\cS}}
            \sum_{a \in \cS} (\bar{r}_a - \ip{a, u^{\star}})^2
      }
      \lesssim
      \frac{\log(\abs{\cS} / \delta)}{\epspriv \cdot \min_{a \in \cS} n_{a}}
  \]
  with probability at least $1 - \delta$.
\end{lemma}
\begin{proof}
    Note that since $R > 1$, we have $\theta^{\star} \in \cB(\bm{0}; R)$.
    From optimality of $u^{\star}$, it follows that
    \begin{align*}
        \epsilon^2 &=
        \frac{1}{\abs{\cS}} \sum_{a \in \cS} (\bar{r}_a - \ip{a, u^{\star}})^2
        \\
                             &\leq
        \frac{1}{\abs{\cS}} \sum_{a \in \cS} (\bar{r}_a - \ip{a, \theta^{\star}})^2 \\
        &=
        \frac{1}{\abs{\cS}} \sum_{a \in \cS} \xi_{a}^2 \\
        &\leq
        \left( \max_{a \in \cS} \abs{\xi_a} \right)^2 \\
        &\lesssim
        \left( \frac{2 \log(\abs{\cS} / \delta)}{\epspriv \min_{a \in \cS} n_{a}} \right)^2,
    \end{align*}

    using~\cref{lemma:max-laplacian-event}. Taking away squares yields the
    desired inequality.
\end{proof}

Continuing, we let $\bar{w}$ be the output of SCRAM with $R = 2$. We have
\begin{align}
    \ip{a, \bar{w} - \theta^{\star}} &=
    \ip{a, \bar{w} - u^{\star}} + \ip{a, u^{\star} - \theta^{\star}} \notag \\
    &\leq
    \norm{a}_{M_n^{-1}} \norm{\bar{w} - u^{\star}}_{M_n} +
    \left( \ip{a, u^{\star}} - (\ip{a, \theta^{\star}} + \xi_a) + \xi_a\right) \notag \\
    &\leq
    \norm{a}_{M_n^{-1}} \norm{\bar{w} - u^{\star}}_{M_n} +
    \abs{\ip{a, u^{\star}} - \bar{r}_a} + \abs{\xi_a}
    \label{eq:scram-plugin-residual}
\end{align}
\begin{lemma}
  \label{lemma:scram-plugin-residual-oracle-part}
  With probability at least $1 - \delta$, we have the following bound
  (uniformly over $a \in \cA$):
  \begin{equation}
    \abs{\ip{a, u^{\star}} - \bar{r}_a} + \abs{\xi_a} \lesssim
    \frac{\log(d \log \log d / \delta) \sqrt{d \log \log d}}{\epspriv \nu n}.
  \end{equation}
\end{lemma}
\begin{proof}
  Condition on the event $\cQ$, which happens with the prescribed probability.
  By optimality of $u^{\star}$ over $\cB^d \ni \theta^{\star}$, we can upper
  bound the first term by
  \begin{align*}
      (\ip{a, u^{\star}} - \bar{r}_a)^2 &\leq
      \sum_{a \in \cS} (\ip{a, u^{\star}} - \bar{r}_a)^2
      \leq
      \sum_{a \in \cS} (\ip{a, \theta^{\star}} - \bar{r}_a)^2 =
      \abs{\cS} \epsilon^2 \lesssim
      \frac{4 \abs{\cS} \log^2(\abs{\cS} / \delta)}{\epspriv^2 \min_{a} n_{a}^2},
  \end{align*}
  using~\cref{lemma:misspecification-error}. Recalling $n_{a} = \max\set{\nu, \pi(a)} \cdot n$, the bound above becomes
  \begin{align}
      \max_{a \in \cS} \abs{\ip{a, u^{\star}} - \bar{r}_a} &\lesssim
      \frac{\log(d \log \log d / \delta) \sqrt{d \log \log d}}{\epspriv \nu n}
      \label{eq:bound-residual-1}
  \end{align}
  At the same time, conditioning on $\cQ$ guarantees that
  \begin{equation}
      \max_{a \in \cS} \abs{\xi_a} \lesssim
      \frac{\log(\frac{d \log \log d}{\delta})}{\epspriv \cdot \nu n}.
      \label{eq:bound-residual-2}
  \end{equation}
  Combining~\cref{eq:bound-residual-1,eq:bound-residual-2} completes the proof.
\end{proof}
With~\cref{lemma:scram-plugin-residual-oracle-part} at hand,
it remains to bound the first term in~\eqref{eq:scram-plugin-residual}.

To that end, we first note that for any $v \in \cA$ the following bound takes hold:
\begin{align}
    \norm{v}^2_{M_n^{-1}} &=
    \biggip{v, \left(\frac{1}{\abs{\cS}} \sum_{a \in \cS} aa^{\T}\right)^{-1} v}
    \notag \\
    &\leq
    \biggip{v, \left( \frac{1}{\abs{\cS}} \sum_{a \in \cS} \pi(a)aa^{\T} \right)^{-1} v} \notag \\
    &\leq
    \abs{\cS}
    \biggip{v, \left( \sum_{a \in \cS} \pi(a) aa^{\T}\right)^{-1} v} \notag \\
    &=
    \abs{\cS} \norm{v}_{M^{-1}(\pi)}^2 \notag \\
    &\leq d^2 \log\log d,
    \label{eq:bound-residual-3}
\end{align}
where the first inequality follows from the properties
\[
    \sum_{a \in \cS} aa^{\T} \succeq
    \sum_{a \in \cS} \pi(a) aa^{\T}, \quad
    \text{and} \quad
    A \succeq B \implies
    \norm{a}_{A^{-1}} \leq \norm{a}_{B^{-1}}
\]
and the last inequality follows from the fact that our coreset construction
guarantees that
\[
  \abs{\cS} \lesssim d \log \log d, \quad \norm{v}^2_{M^{-1}(\pi)} \leq 2d \; \;
  \text{for all $v \in \cA$}.
\]
Finally, we instantiate the bounds from~\cref{theorem:scram} to estimate
$\norm{\bar{w} - u^{\star}}_{M_n}$. Using~\cref{lemma:misspecification-error}
to bound the terms depending on $\epsilon$, it follows that
\begin{equation}
  \epsilon \sqrt{\alpha} + \alpha^{1/8} \sqrt{R \epsilon}
  \left(\frac{\log(\frac{n + d}{\delta})}{n}\right)^{1/8}
  \lesssim
  \frac{\log(\abs{\cS} / \delta) \sqrt{\alpha}}{\epspriv \nu n} +
  \sqrt{
    \frac{\log(\abs{\cS} / \delta)}{\epspriv \nu n}
  } \cdot
  \max\set{\alpha, \frac{\log(\frac{n+d}{\delta})}{n}}^{1/4}
\end{equation}
The terms in~\cref{theorem:scram} depending on $\alpha$
but not $\epsilon$ contribute at most
\begin{align*}
  \alpha \sigma + \sqrt{\sigma} \alpha^{3/8} \bigg(\frac{\log(\frac{n+d}{\delta})}{n}\bigg)^{1/8}
  + \alpha^{1/4} \bigg(\frac{\log(\frac{n+d}{\delta})}{n}\bigg)^{1/4}
\end{align*}
to the error. Finally, putting everything together yields
\begin{align}
    \abs{\ip{a, \bar{w} - \theta^{\star}}} &\leq
    \norm{a}_{M_n^{-1}} \norm{\bar{w} - u^{\star}}_{M_n} +
    \max_{a \in \cA} \abs{\ip{a, u^{\star}} - \bar{r}_a} + \abs{\xi_{a}} \notag \\
                                      &\lesssim
    \begin{aligned}[t]
    & d \sqrt{\log \log d} \left(
            \alpha \sigma + (\sqrt{\sigma} + 1) \max\set{
                \alpha, \frac{\log(\frac{n+d}{\delta})}{n}
            }^{1/2}
        \right) \\
    &+ d \sqrt{\log \log d} \left(
          \frac{\log(d \log \log d / \delta) \sqrt{\alpha}}{\epspriv \nu n} +
            \sqrt{\frac{\log (d \log \log d/ \delta)}{\epspriv \nu n}}
            \max\set{\alpha, \frac{\log(\frac{n + d}{\delta})}{n}}^{1/4}
        \right) \\
    &+ \sigma d \sqrt{\log \log d} \cdot \sqrt{\frac{d + \log(1 / \delta)}{n}}
     + \frac{\log(d \log \log d / \delta) \sqrt{d \log \log d}}{\epspriv \nu n},
    \end{aligned}
    \label{eq:gamma-i-robust}
\end{align}
where $\sigma = \max_{a} \sigma_{a} \lesssim \frac{1}{\sqrt{\nu n}}$.
Before we proceed with regret analysis, we bound the epoch length.

\begin{lemma}
  \label{lemma:total-epoch-length}
  Let $q \in \Nbb_+$ and suppose $n_i = q^i$ at the $i^{\text{th}}$ stage of the
  algorithm. Then we have that
  \[
    \sum_{a \in \cA_{i}} n_{a}^{(i)} \lesssim
    d \log\log d + q^i (1 + \nu d \log \log d).
  \]
\end{lemma}
\begin{proof}
  Dropping the iteration index $i$ for simplicity, recall that
  $n_{a} = \ceil{\max\set{\pi(a), \nu} \cdot n}$. Then
  \begin{align*}
    \sum_{a \in \cA: \pi(a) > 0} n_{a} &\leq
    \sum_{a \in \cA: \pi(a) > 0} (\max\set{\pi(a), \nu} \cdot n + 1) \\
                                       &\leq
                                       \abs{\cS} + n \sum_{a \in \cA: \pi(a) > 0} \max\set{\pi(a), \nu} \\
                                       &\leq
                                       \abs{\cS} + n(1 + \abs{\cS} \nu),
  \end{align*}
  where $\abs{\cS} \lesssim d \log \log d$ is the size of the support of the coreset used.
\end{proof}

\subsubsection{Regret analysis}
We now proceed by analyzing the regret of the algorithm. We let $n_{i} = q^i$
and denote the total epoch length at step $i$ by $m_{i} = \sum_{a} n_{a}^{(i)}$.
Moreover, we note that for any $q > 1$ we have
\[
  q^{i-1} \leq q^{B-1} \implies
  \log\left(\frac{q^{i-1} + d}{\delta}\right) \leq
  \log\left(\frac{T + d}{\delta}\right).
\]

We bound each term in~\cref{eq:gamma-i-robust} separately, conditioning on the
``good'' event where all calls to \textsc{Scram} succeed and the event $\cQ$ from
\eqref{eq:max-laplacian-event} succeeds at each round $i$.

For the first term, we have:
\begin{align}
  \sum_{i = 1}^B m_{i} d \sqrt{d \log \log d} \alpha \sigma &\leq
  \sum_{i = 1}^B m_{i} d \sqrt{d \log \log d} \frac{\alpha}{\sqrt{\nu q^i}} \notag \\
                                                            &\leq
  \sum_{i = 1}^B (d \sqrt{d \log \log d} + q^i(1 + \nu d \log \log d))
  \frac{d \sqrt{d \log \log d} \alpha}{\sqrt{\nu q^{i - 1}}} \notag \\
                                                                                    &\lesssim
  \frac{dq (1 + \nu d \log \log d) \sqrt{d \log \log d} \alpha}{\sqrt{\nu}} \sum_{i = 0}^{B-1}
  \sqrt{q^i} \notag \\
                                                                                    &\lesssim
  \frac{dq (1 + \nu d \log \log d) \sqrt{d \log \log d} \alpha}{\sqrt{\nu}} \cdot
  \frac{q^{B/2} - 1}{q^{1/2} - 1}.
  \label{eq:regret-term-i}
\end{align}
Given that $\sigma \lesssim (\nu n_i)^{-1/2}$, letting $\sqrt{\sigma} + 1 \lesssim 1$ we obtain
for the second term in~\eqref{eq:gamma-i-robust}:
\begin{align}
  & \sum_{i=1}^B m_{i} d \sqrt{d \log\log d} (\sqrt{\sigma} + 1)
    \max\set{\alpha, \frac{\log(\frac{n_{i-1} + d}{\delta})}{n_{i-1}}}^{1/2} \notag \\
  &\lesssim
    dq(1 + \nu d \log \log d) \sqrt{d \log \log d} \sum_{i = 1}^B q^{i-1}
    \max\set{\alpha, \frac{\log(\frac{T + d}{\delta})}{q^{i-1}}}^{1/2} \notag \\
  &\lesssim
  dq(1 + \nu d \log \log d) \sqrt{d \log \log d} \sum_{j = 0}^{B-1}
  \max\set{q^{j} \sqrt{\alpha}, \sqrt{q^{j} \log((T + d)/\delta)}} \notag \\
  &\lesssim
  dq(1 + \nu d \log \log d) \sqrt{d \log \log d} \cdot \max\set{
    T \sqrt{\alpha},
    \log^{1/2}\left(\frac{T+d}{\delta}\right)
    \cdot \frac{q^{B/2} - 1}{q^{1/2} - 1}}
    \label{eq:regret-term-ii}
\end{align}

The third term in~\eqref{eq:gamma-i-robust} is simpler to analyze. In particular, we have:
\begin{align}
  \sum_{i = 1}^B m_{i} d \sqrt{\log \log d} \cdot
    \frac{\log(d \log \log d / \delta) \sqrt{\alpha}}{\epspriv \nu q^{i-1}} &\lesssim
  \frac{dq (1 + \nu d \log \log d) \sqrt{\alpha d \log \log d}}{\epspriv \nu}
  \sum_{i = 0}^{B-1} 1 \notag \\
                                                                                                                    &\leq
  \frac{B dq (1 + \nu d \log \log d) \sqrt{\alpha d \log \log d}}{\epspriv \nu}
  \label{eq:regret-term-iii}
\end{align}

For the fourth term in~\eqref{eq:gamma-i-robust}, we obtain:
\begin{align}
  & \sum_{i = 1}^B m_{i} d \sqrt{\log \log d} \sqrt{\frac{\log (d \log \log d / \delta)}{\epspriv \nu q^{i-1}}}
  \max\set{\alpha, \frac{\log(\frac{q^{i-1} + d}{\delta})}{q^{i-1}}}^{1/4} \notag \\
  & \lesssim
  dq(1 + \nu d \log \log d) \sqrt{\frac{\log(d \log \log d / \delta)}{\epspriv \nu}}
  \sum_{i = 0}^{B - 1} \max\set{\alpha q^{2j}, \log((T + d) / \delta) q^j}^{1/4} \notag \\
  &\leq
  dq(1 + \nu d \log \log d) \sqrt{\frac{\log(d \log \log d / \delta)}{\epspriv \nu}}
  \max\set{\sqrt{\alpha} \cdot \frac{q^{B/2} - 1}{q^{1/2} - 1},
           \log^{1/4}\left(\frac{T+d}{\delta}\right) \cdot \frac{q^{B/4} - 1}{q^{1/4} - 1}}.
  \label{eq:regret-term-iv}
\end{align}
Again using $\sigma \lesssim (\nu n)^{-1/2}$, we obtain for the fifth term in~\eqref{eq:gamma-i-robust}:
\begin{align}
  \sum_{i=1}^B m_{i} \sigma d \sqrt{d \log \log d} \sqrt{\frac{d + \log(1 / \delta)}{n_i}} &\lesssim
  dq(1 + \nu d \log \log d)\sqrt{d \log \log d}
  \sum_{i = 0}^{B-1} \sqrt{q^{i} \cdot \frac{d + \log(1 / \delta)}{\nu q^i}} \notag \\
                                                                                           &\leq
  dq(1 + \nu d \log \log d)\sqrt{\frac{d \log \log d (d + \log(1 / \delta))}{\nu}}
  \cdot B
  \label{eq:regret-term-v}
\end{align}
Finally, for the sixth and final term in~\eqref{eq:gamma-i-robust}, we have the regret bound:
\begin{align}
\sum_{i=1}^B m_{i} \frac{\log(d \log \log d / \delta) \sqrt{d \log \log d}}{\epspriv \nu n} \lesssim
\frac{Bqd(1 + \nu d \log \log d)\sqrt{d \log \log d} \log(d \log \log d / \delta)}{\epspriv \nu}.
\label{eq:regret-term-vi}
\end{align}

Now, suppose that $q = T^{1/B}$ and $B \geq c\log(T)$. For any $\omega > 0$, we have
\[
  q^{\omega} = (e^{\log T^{1/B}})^{\omega} \leq
  (e^{\log T^{1/(c\log T)}})^{\omega} =
  e^{\frac{\omega}{c}}.
\]
This implies the following bounds:
\begin{align}
  \eqref{eq:regret-term-i} &= \tilde{O}\left(
    \alpha \cdot T^{1/B} d^{5/2} \sqrt{T}
  \right) \\
  \eqref{eq:regret-term-ii} &=
    \tilde{O}\left(
      T^{1/B} d^{5/2}
    \max\set{T \sqrt{\alpha}, \sqrt{T}}
  \right) \\
  \eqref{eq:regret-term-iii} &=
  \tilde{O}\left(
    \frac{B T^{1/B} d^{5/2}}{\epspriv} \sqrt{\alpha}
  \right) \\
  \eqref{eq:regret-term-iv} &=
  \tilde{O}\left(
    T^{1/B} d^{3/2} \max\set{
      \sqrt{\frac{\alpha T}{\epspriv}}, \frac{T^{1/4}}{\epspriv^{1/2}}
    }
  \right) \\
  \eqref{eq:regret-term-v} &=
  \tilde{O}\left(
    B d^3 
  \right) \\
  \eqref{eq:regret-term-vi} &=
  \tilde{O}\left(
    \frac{B d^{5/2}}{\epspriv}
  \right)
\end{align}

{\color{red} \textbf{TODO}s:
\begin{enumerate}
    \item Add differences with:
    \begin{enumerate}
        \item The dependence on corruption appearing in~\cite{BLKS21}. [\textbf{DONE}]
        \item The DP algorithms presented in~\cite{HGFD22}.
    \end{enumerate}
    \item For central-DP, try the following:
    \begin{enumerate}
        \item Change every item by the allowed range.
        \item Check if the outputs of the algorithm changed by a lot.
        \item If they did, report the empirical average.
    \end{enumerate}
    That makes the algorithm fail with some probability but does not forego privacy.

    \textbf{Note}: changing items also changes the oracle least squares solution. How to proceed?
    
    \item Try a version where we form the coreset and keep all the vectors to form the Gram
      matrix, but only collect rewards from a uniform random subset. This is to address
      ``pure exploration'' settings, where $d$ can be much larger than the number of rounds $T$.

    \item \textbf{Idea}: consider a version with ``compression'', wherein every client returns
      \[
        r_{a} := \Delta \cdot \left(\floor{\frac{\ip{a, \theta^{\star}} + \tau}{\Delta}} + \frac{1}{2}\right),
        \tau_{a} \sim \mathrm{Unif}(-\Delta/2, \Delta/2),
      \]
      i.e., quantization with dithering. What can we learn (privately / robustly)? It is well known that
      \[
        \expec[\tau]{r_{a}} = \ip{a, \theta^{\star}}.
      \]

\end{enumerate}
}
